# Supplementary material for: On the dynamics of a collapsing bubble in contact with a rigid wall
Source: arXiv:2401.05567 source file (2024-01-10)
Supplement: Supplementary file 1 [file supplimentary.tex]

\documentclass{article}
\title{Captions for movies}
\date{\vspace{-5ex}}
\begin{document}
\maketitle

\noindent{\bf Movie 1}: The asymmetric collapse of spherical cap bubble with initial contact angle of 120 degrees, $Re = 5000$ and $We = 1000$ Left: A rendered video of interface. Right: The inverted RdBu colour map of non dimensional velocity magnitude $|\mathbf{u}|/U_c \in (0,1)$ with blue = 0 and red = 1, and the interface is represented with black curve.\\
{\bf Movie 2}: The asymmetric collapse of spherical cap bubble with initial contact angle of 75 degrees, $Re = 5000$ and $We = 1000$ Left: A rendered video of interface. Right: The inverted RdBu colour map of non dimensional velocity magnitude $|\mathbf{u}|/U_c \in (0,1)$ with blue = 0 and red = 1, and the interface is represented with black curve.\\
{\bf Movie 3}: The experiment of flat bubble collapse with ink to visualise vortex formation and its evolution where it travels to long distances in direction opposite to wall and eventually interacts with free-surface leading to long range effects.

\end{document}
